# Supplementary material for: Self-Supervised Similarity Learning for Digital Pathology
Source: arXiv:1905.08139 source file (2020-01-13)
Supplement: Supplementary file 1 [file supp_material.tex]

% This is samplepaper.tex, a sample chapter demonstrating the
% LLNCS macro package for Springer Computer Science proceedings;
% Version 2.20 of 2017/10/04
% %
% \documentclass[runningheads]{llncs}
% %
% \usepackage{graphicx}
% \usepackage{placeins}
% \usepackage{bbding}
% \usepackage{amsfonts}
% % Used for displaying a sample figure. If possible, figure files should
% % be included in EPS format.
% %
% % If you use the hyperref package, please uncomment the following line
% % to display URLs in blue roman font according to Springer's eBook style:
% % \renewcommand\UrlFont{\color{blue}\rmfamily}
% \graphicspath{{Images/}}
% \begin{document}
% %

% \begin{figure}[t]

%   \centering
%   \centerline{\includegraphics[width=1.0\linewidth]{}}
  
% \caption{...
% }
% \label{peliGAN}
% %
% \end{figure}

% %
% \end{document}
